# Supplementary material for: Towards Adaptive Human-centric Video Anomaly Detection: A Comprehensive Framework and A New Benchmark
Source: arXiv:2408.14329 source file (2025-03-19)
Supplement: Supplementary file 1 [file X_suppl.tex]

\clearpage
\setcounter{page}{1}
\maketitlesupplementary

The supplementary materials include comprehensive details regarding the architectural and training hyperparameters employed in the various algorithmic benchmarking conducted on HuVAD (\cref{sec:benchmark} and \cref{sec:continual}). Additionally, it includes details of HuVAD-C statistics and detailed UCAL step-by-step results. These details are provided to ensure the reproducibility of the findings. All training and testing were conducted on a server equipped with 2xEPYC 7513 processors and 3xNvidia A6000 GPUs with 256GB of memory and an Ubuntu 22.04 operating system. Each trained model has its own packages and libraries with specific versions and we have used the same original setup from their official repositories without any changes to ensure correct reproducibility. 
% 
% To split the supplementary pages from the main paper, you can use \href{https://support.apple.com/en-ca/guide/preview/prvw11793/mac#:~:text=Delete%20a%20page%20from%20a,or%20choose%20Edit%20%3E%20Delete).}{Preview (on macOS)}, \href{https://www.adobe.com/acrobat/how-to/delete-pages-from-pdf.html#:~:text=Choose%20%E2%80%9CTools%E2%80%9D%20%3E%20%E2%80%9COrganize,or%20pages%20from%20the%20file.}{Adobe Acrobat} (on all OSs), as well as \href{https://superuser.com/questions/517986/is-it-possible-to-delete-some-pages-of-a-pdf-document}{command line tools}.

\section{HuVAD Standard Benchmark (HuVAD-S) Setup and Hyperparameters}
\label{sec:benchmarking}

The intricate training hyperparameters for each benchmarked model, including MPED-RNN \cite{morais2019learning}, GEPC \cite{markovitz2020graph}, STG-NF \cite{Hirschorn_2023_ICCV}, and TSGAD \cite{noghre2024exploratory}, are provided in detail in  \cref{tab:hyper}. Furthermore, within this section, additional details are elucidated to enhance reproducibility.

% Please add the following required packages to your document preamble:
% \usepackage{booktabs}
% \usepackage{multirow}
\begin{table*}[]
\centering

% \resizebox{0.85\textwidth}{!}{%
\begin{tabular} {@{}p{3.5cm}>{\centering\arraybackslash}p{1.5cm}>{\centering\arraybackslash}p{1cm}>{\centering\arraybackslash}p{1.5cm}>{\centering\arraybackslash}p{1cm}>{\centering\arraybackslash}p{1.5cm}>{\centering\arraybackslash}p{2cm}@{}}
\toprule \toprule
                                                                   & \textbf{Camera}                        & \textbf{LR} & \textbf{DR} & \textbf{WD} & \textbf{\# Epoch} & \textbf{Batch Size} \\ \midrule
\multicolumn{1}{c|}{\multirow{8}{*}{\textbf{MPED-RNN}}}            & \multicolumn{1}{c|}{\textbf{C0}}       & $1e-3$      & -           & -           & 5                 & 256                 \\
\multicolumn{1}{c|}{}                                              & \multicolumn{1}{c|}{\textbf{C1}}       & $1e-3$      & -           & -           & 5                 & 256                 \\
\multicolumn{1}{c|}{}                                              & \multicolumn{1}{c|}{\textbf{C2}}       & $1e-3$      & -           & -           & 5                 & 256                 \\
\multicolumn{1}{c|}{}                                              & \multicolumn{1}{c|}{\textbf{C3}}       & $1e-3$      & -           & -           & 5                 & 256                 \\
\multicolumn{1}{c|}{}                                              & \multicolumn{1}{c|}{\textbf{C4}}       & $1e-3$      & -           & -           & 5                 & 256                 \\
\multicolumn{1}{c|}{}                                              & \multicolumn{1}{c|}{\textbf{C5}}       & $1e-3$      & -           & -           & 5                 & 256                 \\
\multicolumn{1}{c|}{}                                              & \multicolumn{1}{c|}{\textbf{CSC}}      & $1e-3$      & -           & -           & 5                 & 256                 \\
\multicolumn{1}{c|}{}                                              & \multicolumn{1}{c|}{\textbf{Combined}} & $1e-3$      & -           & -           & 5                 & 256                 \\ \midrule
\multicolumn{1}{c|}{\multirow{8}{*}{\textbf{GEPC (Pre-training)}}} & \multicolumn{1}{c|}{\textbf{C0}}       & $1e-3$      & 0.3         & $1e-5$      & 10                & 512                 \\
\multicolumn{1}{c|}{}                                              & \multicolumn{1}{c|}{\textbf{C1}}       & $1e-3$      & 0.3         & $1e-5$      & 10                & 512                 \\
\multicolumn{1}{c|}{}                                              & \multicolumn{1}{c|}{\textbf{C2}}       & $1e-3$      & 0.3         & $1e-5$      & 10                & 512                 \\
\multicolumn{1}{c|}{}                                              & \multicolumn{1}{c|}{\textbf{C3}}       & $1e-4$      & 0.3         & $1e-5$      & 10                & 512                 \\
\multicolumn{1}{c|}{}                                              & \multicolumn{1}{c|}{\textbf{C4}}       & $1e-4$      & 0.3         & $1e-5$      & 10                & 512                 \\
\multicolumn{1}{c|}{}                                              & \multicolumn{1}{c|}{\textbf{C5}}       & $1e-4$      & 0.3         & $1e-5$      & 10                & 512                 \\
\multicolumn{1}{c|}{}                                              & \multicolumn{1}{c|}{\textbf{CSC}}      & $1e-3$      & 0.3         & $1e-5$      & 10                & 512                 \\
\multicolumn{1}{c|}{}                                              & \multicolumn{1}{c|}{\textbf{Combined}} & $1e-4$      & 0.3         & $1e-5$      & 10                & 512                 \\ \midrule
\multicolumn{1}{c|}{\multirow{8}{*}{\textbf{GEPC (Fine-tuning)}}}  & \multicolumn{1}{c|}{\textbf{C0}}       & $8e-4$      & 0.3         & -           & 25                & 512                 \\
\multicolumn{1}{c|}{}                                              & \multicolumn{1}{c|}{\textbf{C1}}       & $8e-4$      & 0.3         & -           & 25                & 512                 \\
\multicolumn{1}{c|}{}                                              & \multicolumn{1}{c|}{\textbf{C2}}       & $8e-4$      & 0.3         & -           & 25                & 512                 \\
\multicolumn{1}{c|}{}                                              & \multicolumn{1}{c|}{\textbf{C3}}       & $8e-4$      & 0.3         & -           & 25                & 512                 \\
\multicolumn{1}{c|}{}                                              & \multicolumn{1}{c|}{\textbf{C4}}       & $8e-4$      & 0.3         & -           & 25                & 512                 \\
\multicolumn{1}{c|}{}                                              & \multicolumn{1}{c|}{\textbf{C5}}       & $8e-4$      & 0.3         & -           & 25                & 512                 \\
\multicolumn{1}{c|}{}                                              & \multicolumn{1}{c|}{\textbf{CSC}}      & $8e-4$      & 0.3         & -           & 25                & 512                 \\
\multicolumn{1}{c|}{}                                              & \multicolumn{1}{c|}{\textbf{Combined}} & $8e-4$      & 0.3         & -           & 25                & 512                 \\ \midrule
\multicolumn{1}{c|}{\multirow{8}{*}{\textbf{STG-NF}}}              & \multicolumn{1}{c|}{\textbf{C0}}       & $5e-4$      & -           & $5e-5$      & 15                & 256                 \\
\multicolumn{1}{c|}{}                                              & \multicolumn{1}{c|}{\textbf{C1}}       & $5e-4$      & -           & $5e-5$      & 15                & 256                 \\
\multicolumn{1}{c|}{}                                              & \multicolumn{1}{c|}{\textbf{C2}}       & $5e-4$      & -           & $5e-5$      & 15                & 256                 \\
\multicolumn{1}{c|}{}                                              & \multicolumn{1}{c|}{\textbf{C3}}       & $9e-3$      & -           & $5e-5$      & 15                & 256                 \\
\multicolumn{1}{c|}{}                                              & \multicolumn{1}{c|}{\textbf{C4}}       & $5e-4$      & -           & $5e-5$      & 15                & 256                 \\
\multicolumn{1}{c|}{}                                              & \multicolumn{1}{c|}{\textbf{C5}}       & $5e-3$      & -           & $5e-5$      & 15                & 256                 \\
\multicolumn{1}{c|}{}                                              & \multicolumn{1}{c|}{\textbf{CSC}}      & $5e-2$      & -           & $5e-5$      & 15                & 256                 \\
\multicolumn{1}{c|}{}                                              & \multicolumn{1}{c|}{\textbf{Combined}} & $5e-4$      & -           & $5e-5$      & 15                & 256                 \\ \midrule
\multicolumn{1}{c|}{\multirow{8}{*}{\textbf{TSGAD}}}         & \multicolumn{1}{c|}{\textbf{C0}}       & $5e-5$      & 0.3         & $5e-5$      & 20                & 256                 \\
\multicolumn{1}{c|}{}                                              & \multicolumn{1}{c|}{\textbf{C1}}       & $5e-5$      & 0.3         & $5e-5$      & 20                & 256                 \\
\multicolumn{1}{c|}{}                                              & \multicolumn{1}{c|}{\textbf{C2}}       & $5e-5$      & 0.3         & $5e-5$      & 20                & 256                 \\
\multicolumn{1}{c|}{}                                              & \multicolumn{1}{c|}{\textbf{C3}}       & $5e-5$      & 0.3         & $5e-5$      & 20                & 256                 \\
\multicolumn{1}{c|}{}                                              & \multicolumn{1}{c|}{\textbf{C4}}       & $5e-5$      & 0.3         & $5e-5$      & 20                & 256                 \\
\multicolumn{1}{c|}{}                                              & \multicolumn{1}{c|}{\textbf{C5}}       & $5e-5$      & 0.3         & $5e-5$      & 20                & 256                 \\
\multicolumn{1}{c|}{}                                              & \multicolumn{1}{c|}{\textbf{CSC}}      & $5e-5$      & 0.3         & $5e-5$      & 20                & 256                 \\
\multicolumn{1}{c|}{}                                              & \multicolumn{1}{c|}{\textbf{Combined}} & $5e-5$      & 0.3         & $5e-5$      & 20                & 256                              \\ \bottomrule \bottomrule
\end{tabular}
\caption{Comprehensive hyperparameters utilized for benchmarking MPED-RNN \cite{morais2019learning}, GEPC \cite{markovitz2020graph}, STG-NF \cite{Hirschorn_2023_ICCV}, and TSGAD \cite{noghre2024exploratory} on the HuVAD-S. The corresponding results are presented in \cref{tab:benchmark}. LR, DR and WD indicate Learning Rate, Dropout Rate and Weight Decay. }
\label{tab:hyper}
\end{table*}

\textbf{MPED-RNN \cite{morais2019learning}}: In training MPED-RNN for all cameras, we established the input window length at 30 frames or 1 second, with reconstruction and prediction lengths set to 12 and 6, respectively. The architectural choice leaned towards the Gated Recurrent Unit (GRU) cell type, as it was identified as the optimal model in the original research. In alignment with the original study, no regularization techniques were applied during training. 

\textbf{GEPC \cite{markovitz2020graph}}: The input window size remains consistent at 30 frames or 1 second. Throughout all training sessions, we employed the Spatial-Attention Graph Convolution architecture introduced in the original research. Given our specific focus on pose-based anomaly detection, we disabled pixel patches and exclusively utilized pose information. The training process for this model comprises two distinct phases. Initially, the model undergoes pre-training, which involves training the autoencoder. Subsequently, in the fine-tuning step, the encoder and the clustering layer are optimized jointly.

\textbf{STG-NF \cite{Hirschorn_2023_ICCV}}: We utilized the unsupervised setting outlined in the original research, given our focus on unsupervised anomaly detection. Furthermore, we calibrated the prior distribution to $N(3,I)$, in accordance with the setup advocated in the original work. In our benchmarking, the input window size is maintained at 30 frames or 1 second. 

\textbf{TSGAD \cite{noghre2024exploratory}}: As the focus of our paper is on pose-based VAD, we only use the pose branch of TSGAD which uses a Variational Autoencoder (VAE). In the VAE branch, we adhere to the 30 frames or 1 second input window size.

\section{Unsupervised Continual Anomaly Learning Setup and Hyperparameteres}

As discussed in \cref{sec:continual}, an additional data split namely the HuVAD Continual (HuVAD-C) benchmark was introduced for the continual learning benchmark to more accurately simulate real-world scenarios. All the statistics for the HuVAD-C training and test sets can be seen in \cref{tab:continual_set}. The primary objective of this split is to mimic streaming data, where the occurrence of anomalous activities is relatively rare, reflecting real-world conditions. To achieve this, we incorporated less than 1\% anomalous data into the continual training set. The test set was adjusted to achieve a balanced distribution, with an approximately 1:1 ratio of normal to anomalous frames, ensuring that metrics such as AUC-ROC and AUC-PR provide more meaningful insights. The normal frames removed during this process were subsequently added to the streaming training set. 

For training TSGAD \cite{noghre2024exploratory} and STG-NF \cite{Hirschorn_2023_ICCV}, we employed hyperparameters consistent with those detailed in \cref{sec:benchmarking}, in alignment with the models' original configurations. Both models were initially pretrained on the SHT \cite{liu2018future} dataset, with the window size set to 1 second (equivalent to 24 frames) and a stride of 6. During continual learning, both models were trained using a batch size of 256 and a learning rate of $0.005$, over 10 epochs for each of the 9 continual learning steps. Table \ref{tab:continual} summarizes the result over 9 steps for all seven cameras. Additionally, we present comprehensive metrics for each of the 9 continual learning steps, corresponding to Figure 4 in the original manuscript. These detailed results are provided in Tables \ref{tab:c0}, \ref{tab:c1}, \ref{tab:c2}, \ref{tab:c4}, \ref{tab:c5} and \ref{tab:csc} covering all seven camera setups.

\begin{table*}[]
\centering
\begin{tabular}{ccccccccc}
\hline \hline
\multicolumn{9}{c}{\textbf{Number of Frames with Pose}} \\ \hline
\textbf{} & \multicolumn{4}{c}{\textbf{Continual Train Set}} & \multicolumn{4}{c}{\textbf{Continual Test Set}} \\ \hline
\textbf{} & \textbf{Total} & \textbf{Normal} & \textbf{Anomalous} & \textbf{Anomaly} & \textbf{Total} & \textbf{Normal} & \textbf{Anomalous} & \textbf{Anomaly} \\ 
\textbf{} &  &  &  & \textbf{Percentage} &  &  &  & \textbf{Percentage} \\ \hline
\multicolumn{1}{c|}{\textbf{C0}} & 487,835 & 483,220 & 4,615 & \multicolumn{1}{c|}{0.95} & 52,145 & 26,093 & 26,052 & 49.96 \\
\multicolumn{1}{c|}{\textbf{C1}} & 796,860 & 791,186 & 5,674 & \multicolumn{1}{c|}{0.71} & 57,120 & 28,597 & 28,523 & 49.93 \\
\multicolumn{1}{c|}{\textbf{C2}} & 787,301 & 780,420 & 6,881 & \multicolumn{1}{c|}{0.87} & 50,592 & 25,300 & 25,292 & 49.99 \\
\multicolumn{1}{c|}{\textbf{C3}} & 1,260,314 & 1,251,189 & 9,125 & \multicolumn{1}{c|}{0.72} & 31,604 & 15,818 & 15,786 & 49.95 \\
\multicolumn{1}{c|}{\textbf{C4}} & 449,686 & 447,918 & 1,768 & \multicolumn{1}{c|}{0.39} & 74,482 & 37,274 & 37,208 & 49.95 \\
\multicolumn{1}{c|}{\textbf{C5}} & 690,730 & 686,435 & 4,295 & \multicolumn{1}{c|}{0.62} & 56,621 & 28,353 & 28,268 & 49.92 \\
\multicolumn{1}{c|}{\textbf{CSC}} & 558,492 & 555,223 & 3,269 & \multicolumn{1}{c|}{0.58} & 56,644 & 28,343 & 28,301 & 49.96 \\
\hline \hline
\end{tabular}%
\caption{HuVAD-C training and test set characteristics. Less than 1\% of the training data is anomalous to mimic real-world scenarios. The test set is edited to be balanced with an approximate 1:1 ratio of normal to anomalous frames to make metrics such as AUC-ROC and AUC-PR more informative.}
\label{tab:continual_set}
\end{table*}

\begin{table*}[]
\centering
\begin{tabular}{cc|cccccccc}
\hline \hline
\textbf{Model} & \textbf{Case} & \textbf{AUC-ROC} & \textbf{AUC-PR} & \textbf{EER} & \multicolumn{1}{c|}{\textbf{10ER}} & \textbf{AUC-ROC} & \textbf{AUC-PR} & \textbf{EER} & \textbf{10ER} \\ \hline
\textbf{} & \textbf{} & \multicolumn{4}{c|}{\textbf{C0}} & \multicolumn{4}{c}{\textbf{C1}} \\ \hline
\multicolumn{1}{c|}{\multirow{4}{*}{\textbf{TSGAD}}} & Baseline & 54.32 & 51.59 & 0.46 & \multicolumn{1}{c|}{0.84} & 54.73 & 54.34 & 0.45 & {\underline{ 0.86}} \\
\multicolumn{1}{c|}{} & UCAL Average & 53.06 & 54.40 & 0.48 & \multicolumn{1}{c|}{0.87} & {\underline{57.42}} & 57.52 & {\underline{0.44}} & 0.87 \\
\multicolumn{1}{c|}{} & Normal Training & \textbf{58.19} & \textbf{61.14} & \textbf{0.45} & \multicolumn{1}{c|}{{\underline{0.84}}} & 55.17 & {\underline{60.25}} & 0.47 & 0.88 \\
\multicolumn{1}{c|}{} & UCAL Best & {\underline{56.45}} & {\underline{60.72}} & {\underline{0.46}} & \multicolumn{1}{c|}{\textbf{0.82}} & \textbf{60.81} & \textbf{63.77} & \textbf{0.42} & \textbf{0.82} \\ \hline
\multicolumn{1}{c|}{\multirow{4}{*}{\textbf{STG-NF}}} & Baseline & 54.30 & 52.21 & 0.46 & \multicolumn{1}{c|}{0.84} & 43.50 & 44.32 & 0.53 & 0.93 \\
\multicolumn{1}{c|}{} & UCAL Average & {\underline{57.39}} & {\underline{58.86}} & {\underline{0.45}} & \multicolumn{1}{c|}{{\underline{0.82}}} & 47.70 & 48.35 & 0.52 & {\underline{0.88}} \\
\multicolumn{1}{c|}{} & Normal Training & 56.54 & 57.40 & 0.46 & \multicolumn{1}{c|}{0.84} & \textbf{48.47} & \textbf{50.01} & \textbf{0.51} & 0.91 \\
\multicolumn{1}{c|}{} & UCAL Best & \textbf{57.94} & \textbf{60.25} & \textbf{0.44} & \multicolumn{1}{c|}{\textbf{0.82}} & {\underline{48.30}} & {\underline{49.42}} & {\underline{0.52}} & \textbf{0.87} \\ \hline
\textbf{} &  & \multicolumn{4}{c|}{\textbf{C2}} & \multicolumn{4}{c}{\textbf{C3}} \\ \hline
\multicolumn{1}{c|}{\multirow{4}{*}{\textbf{TSGAD}}} & Baseline & 58.31 & 57.64 & 0.43 & \multicolumn{1}{c|}{0.83} & 60.80 & 57.16 & 0.42 & 0.75 \\
\multicolumn{1}{c|}{} & UCAL Average & {\underline{62.09}} & 61.73 & {\underline{0.42}} & \multicolumn{1}{c|}{0.76} & 68.53 & 68.45 & 0.36 & 0.76 \\
\multicolumn{1}{c|}{} & Normal Training & 61.57 & {\underline{62.10}} & 0.44 & \multicolumn{1}{c|}{{\underline{0.76}}} & {\underline{69.57}} & {\underline{71.62}} & {\underline{0.35}} & {\underline{0.72}} \\
\multicolumn{1}{c|}{} & UCAL Best & \textbf{62.88} & \textbf{63.22} & \textbf{0.41} & \multicolumn{1}{c|}{\textbf{0.73}} & \textbf{73.47} & \textbf{75.93} & \textbf{0.32} & \textbf{0.70} \\ \hline
\multicolumn{1}{c|}{\multirow{4}{*}{\textbf{STG-NF}}} & Baseline & 50.85 & 52.91 & 0.48 & \multicolumn{1}{c|}{0.91} & 43.41 & 44.96 & 0.54 & 0.93 \\
\multicolumn{1}{c|}{} & UCAL Average & {\underline{59.98}} & {\underline{60.56}} & {\underline{0.43}} & \multicolumn{1}{c|}{{\underline{0.84}}} & {\underline{51.09}} & {\underline{50.50}} & {\underline{0.49}} & {\underline{0.90}} \\
\multicolumn{1}{c|}{} & Normal Training & 57.86 & 59.94 & 0.44 & \multicolumn{1}{c|}{0.88} & 46.96 & 47.45 & 0.51 & 0.92 \\
\multicolumn{1}{c|}{} & UCAL Best & \textbf{61.97} & \textbf{62.42} & \textbf{0.41} & \multicolumn{1}{c|}{\textbf{0.81}} & \textbf{53.11} & \textbf{52.93} & \textbf{0.48} & \textbf{0.84} \\ \hline
\textbf{} & \textbf{} & \multicolumn{4}{c|}{\textbf{C4}} & \multicolumn{4}{c}{\textbf{C5}} \\ \hline
\multicolumn{1}{c|}{\multirow{4}{*}{\textbf{TSGAD}}} & Baseline & 44.05 & 48.64 & 0.51 & \multicolumn{1}{c|}{1.00} & {\underline{57.41}} & {\underline{56.59}} & {\underline{0.44}} & {\underline{0.82}} \\
\multicolumn{1}{c|}{} & UCAL Average & {\underline{48.40}} & 56.82 & {\underline{0.48}} & \multicolumn{1}{c|}{1.00} & 54.33 & 55.83 & 0.47 & 0.86 \\
\multicolumn{1}{c|}{} & Normal Training & 47.93 & {\underline{57.27}} & 0.49 & \multicolumn{1}{c|}{{\underline{1.00}}} & 52.19 & 51.01 & 0.47 & 0.88 \\
\multicolumn{1}{c|}{} & UCAL Best & \textbf{49.68} & \textbf{58.37} & \textbf{0.46} & \multicolumn{1}{c|}{\textbf{1.00}} & \textbf{62.95} & \textbf{63.81} & \textbf{0.39} & \textbf{0.81} \\ \hline
\multicolumn{1}{c|}{\multirow{4}{*}{\textbf{STG-NF}}} & Baseline & 37.89 & 40.60 & 0.56 & \multicolumn{1}{c|}{0.88} & 46.48 & 46.58 & 0.52 & 0.88 \\
\multicolumn{1}{c|}{} & UCAL Average & {\underline{40.63}} & {\underline{41.72}} & 0.55 & \multicolumn{1}{c|}{{\underline{0.87}}} & \textbf{53.59} & 53.81 & {\underline{0.48}} & {\underline{0.86}} \\
\multicolumn{1}{c|}{} & Normal Training & 40.62 & 41.67 & {\underline{0.54}} & \multicolumn{1}{c|}{0.90} & 52.87 & \textbf{55.56} & 0.48 & 0.90 \\
\multicolumn{1}{c|}{} & UCAL Best & \textbf{41.40} & \textbf{42.03} & \textbf{0.53} & \multicolumn{1}{c|}{\textbf{0.80}} & \textbf{55.89} & {\underline{55.23}} & \textbf{0.47} & \textbf{0.84} \\ \hline
\textbf{} & \textbf{} & \multicolumn{8}{c}{\textbf{CSC}} \\ \hline
\multicolumn{1}{c|}{\multirow{4}{*}{\textbf{TSGAD}}} & Baseline & \multicolumn{2}{c}{60.10} & \multicolumn{2}{c}{59.90} & \multicolumn{2}{c}{0.41} & \multicolumn{2}{c}{0.83} \\
\multicolumn{1}{c|}{} & UCAL Average & \multicolumn{2}{c}{60.44} & \multicolumn{2}{c}{61.42} & \multicolumn{2}{c}{0.42} & \multicolumn{2}{c}{0.86} \\
\multicolumn{1}{c|}{} & Normal Training & \multicolumn{2}{c}{\textbf{67.15}} & \multicolumn{2}{c}{\textbf{69.14}} & \multicolumn{2}{c}{\textbf{0.35}} & \multicolumn{2}{c}{\textbf{0.82}} \\
\multicolumn{1}{c|}{} & UCAL Best & \multicolumn{2}{c}{{\underline{65.46}}} & \multicolumn{2}{c}{{\underline{67.75}}} & \multicolumn{2}{c}{{\underline{0.36}}} & \multicolumn{2}{c}{{\underline{0.82}}} \\ \hline
\multicolumn{1}{c|}{\multirow{4}{*}{\textbf{STG-NF}}} & Baseline & \multicolumn{2}{c}{49.84} & \multicolumn{2}{c}{48.68} & \multicolumn{2}{c}{0.49} & \multicolumn{2}{c}{\textbf{0.88}} \\
\multicolumn{1}{c|}{} & UCAL Average & \multicolumn{2}{c}{53.90} & \multicolumn{2}{c}{52.96} & \multicolumn{2}{c}{{\underline{0.46}}} & \multicolumn{2}{c}{0.90} \\
\multicolumn{1}{c|}{} & Normal Training & \multicolumn{2}{c}{{\underline{54.55}}} & \multicolumn{2}{c}{{\underline{54.63}}} & \multicolumn{2}{c}{0.47} & \multicolumn{2}{c}{0.90} \\
\multicolumn{1}{c|}{} & UCAL Best & \multicolumn{2}{c}{\textbf{56.90}} & \multicolumn{2}{c}{\textbf{55.71}} & \multicolumn{2}{c}{\textbf{0.44}} & \multicolumn{2}{c}{{\underline{0.89}}} \\ \hline \hline
\end{tabular}%
\caption{UCAL applied to TSGAD \cite{noghre2024exploratory} and STG-NF \cite{Hirschorn_2023_ICCV}. The baseline results are trained on SHT \cite{liu2018future} and tested on HuVAD-C test set and the normal training is the result of conventional training and testing on HuVAD-C train and test sets.}
\label{tab:continual}
\end{table*}

\begin{table*}[]
\centering
\begin{tabular}{ccccccccc}
\hline \hline
 & \multicolumn{8}{c}{\textbf{C0}} \\ \hline
 & \multicolumn{4}{c}{\textbf{TSGAD}} & \multicolumn{4}{c}{\textbf{STG-NF}} \\ \hline
\textbf{} & \textbf{AUC-ROC} & \textbf{AUC-PR} & \textbf{EER} & \textbf{10ER} & \textbf{AUC-ROC} & \textbf{AUC-PR} & \textbf{EER} & \textbf{10ER} \\ \hline
\multicolumn{1}{c|}{\textbf{Baseline}} & 54.32 & 51.59 & 0.46 & \multicolumn{1}{c|}{0.84} & 54.30 & 52.21 & 0.46 & 0.84 \\
\multicolumn{1}{c|}{\textbf{1}} & 56.45 & 60.72 & 0.47 & \multicolumn{1}{c|}{0.87} & 57.49 & 58.78 & 0.46 & 0.82 \\
\multicolumn{1}{c|}{\textbf{2}} & 50.67 & 52.73 & 0.50 & \multicolumn{1}{c|}{0.87} & 57.87 & 59.31 & 0.44 & 0.82 \\
\multicolumn{1}{c|}{\textbf{3}} & 50.10 & 54.72 & 0.50 & \multicolumn{1}{c|}{0.91} & 57.83 & 60.25 & 0.45 & 0.82 \\
\multicolumn{1}{c|}{\textbf{4}} & 56.93 & 57.49 & 0.47 & \multicolumn{1}{c|}{0.83} & 57.95 & 59.57 & 0.45 & 0.83 \\
\multicolumn{1}{c|}{\textbf{5}} & 53.11 & 53.36 & 0.49 & \multicolumn{1}{c|}{0.88} & 57.39 & 59.31 & 0.46 & 0.83 \\
\multicolumn{1}{c|}{\textbf{6}} & 54.12 & 55.11 & 0.46 & \multicolumn{1}{c|}{0.90} & 56.65 & 58.41 & 0.46 & 0.83 \\
\multicolumn{1}{c|}{\textbf{7}} & 54.25 & 57.44 & 0.48 & \multicolumn{1}{c|}{0.89} & 56.44 & 58.21 & 0.46 & 0.83 \\
\multicolumn{1}{c|}{\textbf{8}} & 51.57 & 49.43 & 0.49 & \multicolumn{1}{c|}{0.85} & 57.56 & 58.19 & 0.45 & 0.83 \\
\multicolumn{1}{c|}{\textbf{9}} & 50.35 & 48.62 & 0.49 & \multicolumn{1}{c|}{0.88} & 57.36 & 57.79 & 0.45 & 0.83 \\
\multicolumn{1}{c|}{\textbf{Normal Training}} & 58.20 & 61.15 & 0.45 & \multicolumn{1}{c|}{0.85} & 56.54 & 57.40 & 0.46 & 0.84 \\
\hline \hline
\end{tabular}%
\caption{UCAL step-by-step results for C0, including baseline and normal training results.}
\label{tab:c0}
\end{table*}

\begin{table*}[]
\centering

\begin{tabular}{ccccccccc}
\hline \hline
 & \multicolumn{8}{c}{\textbf{C1}} \\ \hline
 & \multicolumn{4}{c}{\textbf{TSGAD}} & \multicolumn{4}{c}{\textbf{STG-NF}} \\ \hline
\textbf{} & \textbf{AUC-ROC} & \textbf{AUC-PR} & \textbf{EER} & \textbf{10ER} & \textbf{AUC-ROC} & \textbf{AUC-PR} & \textbf{EER} & \textbf{10ER} \\ \hline
\multicolumn{1}{c|}{\textbf{Baseline}} & 54.73 & 54.35 & 0.46 & \multicolumn{1}{c|}{0.86} & 43.59 & 44.32 & 0.54 & 0.93 \\
\multicolumn{1}{c|}{\textbf{1}} & 58.50 & 60.86 & 0.44 & \multicolumn{1}{c|}{0.87} & 47.52 & 49.01 & 0.52 & 0.89 \\
\multicolumn{1}{c|}{\textbf{2}} & 56.17 & 53.45 & 0.44 & \multicolumn{1}{c|}{0.88} & 48.09 & 49.43 & 0.52 & 0.89 \\
\multicolumn{1}{c|}{\textbf{3}} & 58.17 & 55.42 & 0.42 & \multicolumn{1}{c|}{0.88} & 47.79 & 48.60 & 0.53 & 0.89 \\
\multicolumn{1}{c|}{\textbf{4}} & 57.83 & 59.80 & 0.44 & \multicolumn{1}{c|}{0.88} & 47.51 & 48.48 & 0.54 & 0.87 \\
\multicolumn{1}{c|}{\textbf{5}} & 55.83 & 56.31 & 0.44 & \multicolumn{1}{c|}{0.91} & 47.49 & 47.70 & 0.53 & 0.89 \\
\multicolumn{1}{c|}{\textbf{6}} & 57.35 & 58.50 & 0.44 & \multicolumn{1}{c|}{0.88} & 47.73 & 48.29 & 0.53 & 0.89 \\
\multicolumn{1}{c|}{\textbf{7}} & 60.82 & 63.77 & 0.44 & \multicolumn{1}{c|}{0.83} & 47.78 & 48.15 & 0.53 & 0.89 \\
\multicolumn{1}{c|}{\textbf{8}} & 57.79 & 56.29 & 0.44 & \multicolumn{1}{c|}{0.84} & 47.17 & 46.73 & 0.53 & 0.88 \\
\multicolumn{1}{c|}{\textbf{9}} & 54.35 & 53.37 & 0.47 & \multicolumn{1}{c|}{0.86} & 48.31 & 48.78 & 0.52 & 0.89 \\
\multicolumn{1}{c|}{\textbf{Normal Training}} & 55.18 & 60.26 & 0.47 & \multicolumn{1}{c|}{0.89} & 48.48 & 50.01 & 0.52 & 0.91 \\
\hline \hline
\end{tabular}%
\caption{UCAL step-by-step results for C1, including baseline and normal training results.}
\label{tab:c1}
\end{table*}

\begin{table*}[]
\centering

\begin{tabular}{ccccccccc}
\hline \hline
 & \multicolumn{8}{c}{\textbf{C2}} \\ \hline
 & \multicolumn{4}{c}{\textbf{TSGAD}} & \multicolumn{4}{c}{\textbf{STG-NF}} \\ \hline
\textbf{} & \textbf{AUC-ROC} & \textbf{AUC-PR} & \textbf{EER} & \textbf{10ER} & \textbf{AUC-ROC} & \textbf{AUC-PR} & \textbf{EER} & \textbf{10ER} \\ \hline
\multicolumn{1}{c|}{\textbf{Baseline}} & 58.32 & 57.64 & 0.44 & \multicolumn{1}{c|}{0.84} & 50.86 & 52.91 & 0.49 & 0.92 \\
\multicolumn{1}{c|}{\textbf{1}} & 62.27 & 62.59 & 0.42 & \multicolumn{1}{c|}{0.79} & 59.82 & 60.42 & 0.43 & 0.85 \\
\multicolumn{1}{c|}{\textbf{2}} & 62.55 & 61.72 & 0.42 & \multicolumn{1}{c|}{0.77} & 61.00 & 61.68 & 0.42 & 0.84 \\
\multicolumn{1}{c|}{\textbf{3}} & 61.98 & 61.27 & 0.44 & \multicolumn{1}{c|}{0.78} & 61.98 & 62.43 & 0.42 & 0.82 \\
\multicolumn{1}{c|}{\textbf{4}} & 61.65 & 62.48 & 0.43 & \multicolumn{1}{c|}{0.77} & 60.96 & 61.31 & 0.42 & 0.86 \\
\multicolumn{1}{c|}{\textbf{5}} & 62.31 & 60.19 & 0.42 & \multicolumn{1}{c|}{0.73} & 59.75 & 59.84 & 0.43 & 0.84 \\
\multicolumn{1}{c|}{\textbf{6}} & 62.61 & 60.56 & 0.42 & \multicolumn{1}{c|}{0.76} & 58.77 & 58.51 & 0.44 & 0.86 \\
\multicolumn{1}{c|}{\textbf{7}} & 62.89 & 63.22 & 0.42 & \multicolumn{1}{c|}{0.78} & 59.10 & 60.21 & 0.44 & 0.85 \\
\multicolumn{1}{c|}{\textbf{8}} & 61.06 & 61.46 & 0.44 & \multicolumn{1}{c|}{0.78} & 60.58 & 61.17 & 0.42 & 0.84 \\
\multicolumn{1}{c|}{\textbf{9}} & 61.50 & 62.08 & 0.43 & \multicolumn{1}{c|}{0.77} & 57.88 & 59.48 & 0.46 & 0.85 \\
\multicolumn{1}{c|}{\textbf{Normal Training}} & 61.58 & 62.11 & 0.44 & \multicolumn{1}{c|}{0.76} & 57.87 & 59.95 & 0.45 & 0.89 \\
\hline \hline
\end{tabular}%
\caption{UCAL step-by-step results for C2, including baseline and normal training results.}
\label{tab:c2}
\end{table*}

\begin{table*}[]
\centering
\begin{tabular}{ccccccccc}
\hline \hline
 & \multicolumn{8}{c}{\textbf{C3}} \\ \hline
 & \multicolumn{4}{c}{\textbf{TSGAD}} & \multicolumn{4}{c}{\textbf{STG-NF}} \\ \hline
\textbf{} & \textbf{AUC-ROC} & \textbf{AUC-PR} & \textbf{EER} & \textbf{10ER} & \textbf{AUC-ROC} & \textbf{AUC-PR} & \textbf{EER} & \textbf{10ER} \\ \hline
\multicolumn{1}{c|}{\textbf{Baseline}} & 60.81 & 57.16 & 0.43 & \multicolumn{1}{c|}{0.76} & 43.42 & 44.96 & 0.54 & 0.94 \\
\multicolumn{1}{c|}{\textbf{1}} & 61.94 & 56.68 & 0.40 & \multicolumn{1}{c|}{0.92} & 49.03 & 49.06 & 0.51 & 0.92 \\
\multicolumn{1}{c|}{\textbf{2}} & 66.54 & 68.96 & 0.38 & \multicolumn{1}{c|}{0.82} & 53.12 & 52.94 & 0.48 & 0.91 \\
\multicolumn{1}{c|}{\textbf{3}} & 70.37 & 70.81 & 0.35 & \multicolumn{1}{c|}{0.73} & 48.54 & 49.10 & 0.51 & 0.93 \\
\multicolumn{1}{c|}{\textbf{4}} & 65.18 & 59.15 & 0.38 & \multicolumn{1}{c|}{0.71} & 50.03 & 50.59 & 0.50 & 0.94 \\
\multicolumn{1}{c|}{\textbf{5}} & 72.08 & 73.39 & 0.35 & \multicolumn{1}{c|}{0.67} & 50.74 & 51.41 & 0.49 & 0.93 \\
\multicolumn{1}{c|}{\textbf{6}} & 70.53 & 70.91 & 0.35 & \multicolumn{1}{c|}{0.75} & 51.94 & 49.60 & 0.48 & 0.88 \\
\multicolumn{1}{c|}{\textbf{7}} & 67.33 & 69.92 & 0.37 & \multicolumn{1}{c|}{0.79} & 52.46 & 51.16 & 0.48 & 0.87 \\
\multicolumn{1}{c|}{\textbf{8}} & 73.47 & 75.94 & 0.32 & \multicolumn{1}{c|}{0.71} & 51.13 & 49.77 & 0.49 & 0.89 \\
\multicolumn{1}{c|}{\textbf{9}} & 69.38 & 70.33 & 0.36 & \multicolumn{1}{c|}{0.74} & 52.91 & 50.94 & 0.49 & 0.85 \\
\multicolumn{1}{c|}{\textbf{Normal Training}} & 69.58 & 71.62 & 0.35 & \multicolumn{1}{c|}{0.73} & 46.96 & 47.45 & 0.52 & 0.93 \\
\hline \hline
\end{tabular}%
\caption{UCAL step-by-step results for C3, including baseline and normal training results.}
\label{tab:c3}
\end{table*}

\begin{table*}[]
\centering

\begin{tabular}{ccccccccc}
\hline \hline
 & \multicolumn{8}{c}{\textbf{C4}} \\ \hline
 & \multicolumn{4}{c}{\textbf{TSGAD}} & \multicolumn{4}{c}{\textbf{STG-NF}} \\ \hline
\textbf{} & \textbf{AUC-ROC} & \textbf{AUC-PR} & \textbf{EER} & \textbf{10ER} & \textbf{AUC-ROC} & \textbf{AUC-PR} & \textbf{EER} & \textbf{10ER} \\ \hline
\multicolumn{1}{c|}{\textbf{Baseline}} & 60.11 & 59.92 & 0.42 & \multicolumn{1}{c|}{0.84} & 49.84 & 48.68 & 0.50 & 0.89 \\
\multicolumn{1}{c|}{\textbf{1}} & 53.82 & 53.44 & 0.47 & \multicolumn{1}{c|}{0.88} & 56.90 & 55.72 & 0.45 & 0.89 \\
\multicolumn{1}{c|}{\textbf{2}} & 63.64 & 67.46 & 0.41 & \multicolumn{1}{c|}{0.83} & 53.07 & 53.12 & 0.47 & 0.91 \\
\multicolumn{1}{c|}{\textbf{3}} & 65.46 & 62.87 & 0.37 & \multicolumn{1}{c|}{0.85} & 51.21 & 51.33 & 0.49 & 0.91 \\
\multicolumn{1}{c|}{\textbf{4}} & 64.51 & 66.08 & 0.39 & \multicolumn{1}{c|}{0.90} & 54.64 & 53.27 & 0.46 & 0.91 \\
\multicolumn{1}{c|}{\textbf{5}} & 56.91 & 56.81 & 0.44 & \multicolumn{1}{c|}{0.89} & 55.10 & 53.83 & 0.46 & 0.90 \\
\multicolumn{1}{c|}{\textbf{6}} & 54.20 & 56.60 & 0.48 & \multicolumn{1}{c|}{0.86} & 52.99 & 52.32 & 0.48 & 0.92 \\
\multicolumn{1}{c|}{\textbf{7}} & 55.03 & 55.46 & 0.47 & \multicolumn{1}{c|}{0.86} & 54.75 & 52.38 & 0.46 & 0.90 \\
\multicolumn{1}{c|}{\textbf{8}} & 65.11 & 67.76 & 0.38 & \multicolumn{1}{c|}{0.85} & 53.63 & 52.58 & 0.47 & 0.92 \\
\multicolumn{1}{c|}{\textbf{9}} & 65.32 & 66.41 & 0.39 & \multicolumn{1}{c|}{0.83} & 52.86 & 52.11 & 0.47 & 0.92 \\
\multicolumn{1}{c|}{\textbf{Normal Training}} & 67.15 & 69.15 & 0.36 & \multicolumn{1}{c|}{0.83} & 54.55 & 54.63 & 0.47 & 0.90 \\
\hline \hline
\end{tabular}%
\caption{UCAL step-by-step results for C4, including baseline and normal training results.}
\label{tab:c4}
\end{table*}

\begin{table*}[]
\centering

\begin{tabular}{ccccccccc}
\hline \hline
 & \multicolumn{8}{c}{\textbf{C5}} \\ \hline
 & \multicolumn{4}{c}{\textbf{TSGAD}} & \multicolumn{4}{c}{\textbf{STG-NF}} \\ \hline
\textbf{} & \textbf{AUC-ROC} & \textbf{AUC-PR} & \textbf{EER} & \textbf{10ER} & \textbf{AUC-ROC} & \textbf{AUC-PR} & \textbf{EER} & \textbf{10ER} \\ \hline
\multicolumn{1}{c|}{\textbf{Baseline}} & 57.42 & 56.59 & 0.44 & \multicolumn{1}{c|}{0.83} & 46.49 & 46.59 & 0.52 & 0.89 \\
\multicolumn{1}{c|}{\textbf{1}} & 56.60 & 59.14 & 0.46 & \multicolumn{1}{c|}{0.85} & 51.04 & 52.19 & 0.49 & 0.88 \\
\multicolumn{1}{c|}{\textbf{2}} & 60.00 & 62.63 & 0.43 & \multicolumn{1}{c|}{0.88} & 54.58 & 55.24 & 0.48 & 0.86 \\
\multicolumn{1}{c|}{\textbf{3}} & 45.97 & 49.32 & 0.54 & \multicolumn{1}{c|}{0.90} & 51.63 & 52.99 & 0.48 & 0.91 \\
\multicolumn{1}{c|}{\textbf{4}} & 48.01 & 47.66 & 0.52 & \multicolumn{1}{c|}{0.87} & 55.32 & 55.88 & 0.47 & 0.85 \\
\multicolumn{1}{c|}{\textbf{5}} & 48.01 & 47.66 & 0.52 & \multicolumn{1}{c|}{0.87} & 53.66 & 52.92 & 0.49 & 0.86 \\
\multicolumn{1}{c|}{\textbf{6}} & 60.72 & 61.79 & 0.43 & \multicolumn{1}{c|}{0.83} & 53.50 & 53.03 & 0.49 & 0.86 \\
\multicolumn{1}{c|}{\textbf{7}} & 55.27 & 55.47 & 0.47 & \multicolumn{1}{c|}{0.81} & 53.05 & 52.57 & 0.49 & 0.86 \\
\multicolumn{1}{c|}{\textbf{8}} & 62.96 & 63.82 & 0.40 & \multicolumn{1}{c|}{0.83} & 53.65 & 54.58 & 0.49 & 0.86 \\
\multicolumn{1}{c|}{\textbf{9}} & 51.47 & 55.02 & 0.50 & \multicolumn{1}{c|}{0.91} & 55.90 & 54.96 & 0.46 & 0.85 \\
\multicolumn{1}{c|}{\textbf{Normal Training}} & 52.20 & 51.02 & 0.48 & \multicolumn{1}{c|}{0.88} & 52.88 & 55.56 & 0.49 & 0.90 \\
\hline \hline
\end{tabular}%
\caption{UCAL step-by-step results for C5, including baseline and normal training results.}
\label{tab:c5}
\end{table*}

\begin{table*}[]
\centering

\begin{tabular}{ccccccccc}
\hline \hline
 & \multicolumn{8}{c}{\textbf{CSC}} \\ \hline
 & \multicolumn{4}{c}{\textbf{TSGAD}} & \multicolumn{4}{c}{\textbf{STG-NF}} \\ \hline
\textbf{} & \textbf{AUC-ROC} & \textbf{AUC-PR} & \textbf{EER} & \textbf{10ER} & \textbf{AUC-ROC} & \textbf{AUC-PR} & \textbf{EER} & \textbf{10ER} \\ \hline
\multicolumn{1}{c|}{\textbf{Baseline}} & 60.11 & 59.92 & 0.42 & \multicolumn{1}{c|}{0.84} & 49.84 & 48.68 & 0.50 & 0.89 \\ 
\multicolumn{1}{c|}{\textbf{1}} & 53.82 & 53.44 & 0.47 & \multicolumn{1}{c|}{0.88} & 56.90 & 55.72 & 0.45 & 0.89 \\
\multicolumn{1}{c|}{\textbf{2}} & 63.64 & 67.46 & 0.41 & \multicolumn{1}{c|}{0.83} & 53.07 & 53.12 & 0.47 & 0.91 \\
\multicolumn{1}{c|}{\textbf{3}} & 65.46 & 62.87 & 0.37 & \multicolumn{1}{c|}{0.85} & 51.21 & 51.33 & 0.49 & 0.91 \\
\multicolumn{1}{c|}{\textbf{4}} & 64.51 & 66.08 & 0.39 & \multicolumn{1}{c|}{0.90} & 54.64 & 53.27 & 0.46 & 0.91 \\
\multicolumn{1}{c|}{\textbf{5}} & 56.91 & 56.81 & 0.44 & \multicolumn{1}{c|}{0.89} & 55.10 & 53.83 & 0.46 & 0.90 \\
\multicolumn{1}{c|}{\textbf{6}} & 54.20 & 56.60 & 0.48 & \multicolumn{1}{c|}{0.86} & 52.99 & 52.32 & 0.48 & 0.92 \\
\multicolumn{1}{c|}{\textbf{7}} & 55.03 & 55.46 & 0.47 & \multicolumn{1}{c|}{0.86} & 54.75 & 52.38 & 0.46 & 0.90 \\
\multicolumn{1}{c|}{\textbf{8}} & 65.11 & 67.76 & 0.38 & \multicolumn{1}{c|}{0.85} & 53.63 & 52.58 & 0.47 & 0.92 \\
\multicolumn{1}{c|}{\textbf{9}} & 65.32 & 66.41 & 0.39 & \multicolumn{1}{c|}{0.83} & 52.86 & 52.11 & 0.47 & 0.92 \\
\multicolumn{1}{c|}{\textbf{Normal Training}} & 67.15 & 69.15 & 0.36 & \multicolumn{1}{c|}{0.83} & 54.55 & 54.63 & 0.47 & 0.90 \\
\hline \hline
\end{tabular}%
\caption{UCAL step-by-step results for CSC, including baseline and normal training results.}
\label{tab:csc}
\end{table*}
